# Supplementary material for: Efficient Data Shapley for Weighted Nearest Neighbor Algorithms
Source: arXiv:2401.11103 source file (2024-01-20)
Supplement: Supplementary file 1 [file appendix_error_from_approx.tex]

\subsection{Error from Approximation}
\label{appendix:eval-approx}

To visualize the quality of our approximation $\phihatmstar$, Figure \ref{fig:approx_comparison} provides a comparison between the exact Shapley value $\phi_{z_i}$, and approximation $\phihatmstar$, as well as the range introduced by Theorem \ref{thm:error-bound}. The figure shows that the true value always lies within the predicted range, which validates the correctness of our result. 
Moreover, we can see that even though the approximation $\phihatmstar$ represents one end of the predicted range, the true value often comes with remarkable proximity to $\phihatmstar$. 
It empirically reinforces our initial intuition: the building blocks for $\Gil$ (or $\Rim$), $\sum_{s \in [-\wtil_i, 0)} \Fi[t, \ell, s]$ (or $\sum_{s \in [-\wtil_i, -\wtil_m)} \Fi[t, K-1, s]$), are often substantially more restrained in magnitude compared to their counterparts that encompass the entirety of $\wspace$.

\begin{figure}[h]
    \centering
    \includegraphics[width=\columnwidth]{image/shapley_errorbound.pdf}
    \caption{Visualization of the comparison between the exact and approximated WKNN-Shapley value on three OpenML datasets (Fraud, 2DPlanes, and Pol), as well as the interval devised by the approximation algorithm. 
    The red line corresponds to the exact WKNN-Shapley, and the orange line corresponds to the approximated WKNN-Shapley in Definition \ref{def:approxmstar}, which is also \tianhao{TODO}.
    We adjust the value of $\mstar$ so that the error range $\eps = 0.2$ for all three datasets.
    }
    \label{fig:approx_comparison}
\end{figure}
