# Supplementary material for: Efficient Data Shapley for Weighted Nearest Neighbor Algorithms
Source: arXiv:2401.11103 source file (2024-01-20)
Supplement: Supplementary file 2 [file appendix_rebuttal.tex]

\begin{tabular}{@{}ccccc@{}}
\toprule
& \textbf{\begin{tabular}[c]{@{}c@{}}Soft-label\\ KNN-Shapley \\ (Jia et al. (2019))\end{tabular}} & \textbf{\begin{tabular}[c]{@{}c@{}}Hard-label \\ KNN-Shapley \\ (this work)\end{tabular}} & \textbf{\begin{tabular}[c]{@{}c@{}}Exact\\ WKNN-Shapley\\ (this work)\end{tabular}} & \textbf{\begin{tabular}[c]{@{}c@{}}Approximated\\ WKNN-Shapley\\ (this work)\end{tabular}} \\ \midrule
2DPlanes   & 0.48                                                                                         & 0.471                                                                                     & 0.498                                                                                  & 0.511                                                                                         \\
CPU        & 0.549                                                                                        & 0.538                                                                                     & 0.618                                                                                  & 0.604                                                                                         \\
Phoneme    & 0.871                                                                                        & 0.876                                                                                     & 0.911                                                                                  & 0.907                                                                                         \\
Fraud      & 0.449                                                                                        & 0.449                                                                                     & 0.453                                                                                  & 0.493                                                                                         \\
Creditcard & 0.498                                                                                        & 0.502                                                                                     & 0.556                                                                                  & 0.569                                                                                         \\
% Vehicle    & 0.573                                                                                        & 0.578                                                                                     & 0.658                                                                                  & 0.698                                                                                         \\
% Click      & 0.433                                                                                        & 0.456                                                                                     & 0.462                                                                                  & 0.507                                                                                         \\
% Wind       & 0.876                                                                                        & 0.938                                                                                     & 0.938                                                                                  & 0.938                                                                                         \\
% Pol        & 0.556                                                                                        & 0.444                                                                                     & 0.609                                                                                  & 0.6  \\  
\bottomrule                                                                                      
\end{tabular}
